# Supplementary material for: Learning To Count Everything
Source: arXiv:2104.08391 source file (2021-04-16)
Supplement: Supplementary file 1 [file supplementary.tex]

\section{Overview}
 In this Supplementary submission, we provide details related to the FamNet architecture in  \Sref{details}. Additional images from the FSC-147 dataset are shown in \Sref{dataset-images}. We present additional qualitative results on images from the validation and test splits of FSC-147 dataset in \Sref{dataset-images-quali}.
 \newline
\newline
\subsection{Ablation Study on the losses}
\setlength{\tabcolsep}{10pt}
\begin{table}[!t]
%\vskip 0.1in
\centering
\begin{tabular}{crr}
\toprule
Adaptation Loss & MAE & RMSE \\
\midrule 
None & 25.48 & 79.39\\
Perturbation & 25.16 & 79.52 \\
Mincount & 25.15 & 78.87 \\
Perturbation $+$ Mincount & 24.97 & 79.34\\
\bottomrule 
\end{tabular}
\vskip -0.1in
\caption{\textcolor{blue}{entire table}{Evaluating the usefulness of the Perturbation and Mincount losses on Validation set of FSC147}. Using both Perturbation and Mincount losses leads to the best results in terms of MAE metric.
\label{tab:Losses}}
\end{table}

\subsection{Comparison with Few-Shot Approaches on Non-Imagenet subset of FSC147}
Since FamNet contains an Imagenet pretrained Resnet-50 backbone for feature extraction, one may argue that some of the classes in the validation and test split may not be truly unseen, as they may appear in Imagenet. 
\setlength{\tabcolsep}{2pt}
\begin{table}[!tb]
\vskip 0.1in
\centering
\begin{tabular}{lcccc}
\toprule
          &  \multicolumn{2}{c}{ Val Set} &  \multicolumn{2}{c}{ Test Set} \\
         \cmidrule(lr){2-3} \cmidrule(lr){4-5} 
    Method &  MAE          & RMSE    & MAE          & RMSE         \\

\midrule 
Mean & 53.18 & 124.27 & 47.55 & 147.67 \\
Median & 48.44 & 129.40 & 47.73 & 152.46 \\
%{\small pre-trained few-shot detector}\cite{kang2019few} & 50.76 & 126.18 & 44.16 & 146.76 \\
Few-shot detector  \cite{kang2019few} & 46.43  & 111.58 & 41.64 & 141.04 \\
FSOD few-Shot detector \cite{fan2020few} & 36.24 & 114.82 & 32.53  & 140.65 \\
pre-trained GMN \cite{lu2018class} & 60.33 &  137.48 & 62.64 & 159.62 \\
GMN \cite{lu2018class} & 29.77 & 88.21 & 26.36 & 124.50  \\
MAML \cite{finn2017model} & 29.55 & 87.59 & 26.84  & 110.98 \\
%FamNet (Proposed)   & \textbf{26.80} & \textbf{73.83} & \textbf{24.63} & \textbf{102.28}  \\
FamNet (Proposed)   & \textbf{24.97} & \textbf{79.34} & \textbf{21.87} & \textbf{100.22}  \\
\bottomrule 
\end{tabular}
\vskip -0.1in
\caption{Comparing FamNet with competing approaches on Non-Imagenet classes from the validation and test splits.  FamNet has the lowest MAE and RMSE on both validation and test sets.\vr{Do the eval on non imagenet classes}
\label{tab:baselineNonImagenet}}
\end{table}

 \section{Arhictecture Details for FamNet}\label{details}
 As described in the main paper, FamNet architecture consists of two key modules: 1) multi-scale feature extraction module 2) density prediction module. The feature extraction module consists of the first four blocks from a pre-trained ResNet-50
backbone(the parameters of these blocks are frozen during training).
\newline
\newline
The density prediction module has the following architecture:
Conv7-196, Upsampling-2, Conv5-128, Upsampling-2, Conv3-64, Upsampling-2, Conv1-32, Conv1-1. Here, ConvX-Y implies a convolution layer having Y filters with \htimesw{X}{X} kernel size. Upsampling-2 refers to the bilinear interpolation layer which upsamples the input to twice its size. Upsampling-2 layer does not have any learnable parameters. We use ReLU nonlinearity after each convolution layer.
\newline
\newline
\section{Additional Images from the FSC-147 Dataset}\label{dataset-images}
In \Fref{fig:annotation_examples1}, we present few representative images from our FSC-147 dataset. We present images from the following visual categories: tomatoes, birds, marbles, lipstick, alcohol bottles, cans, chair, beads, zebras, coffee beans, cashew nuts, potatoes, kidney beans, bottle caps and watermelon. We also show the dot annotations and the exemplars for all the images. The dot annotations and the exemplars are shown in red and blue respectively. As can be seen from the images, the number of objects in the images varies widely, some images contain a dozen of objects while some contain thousands. Some of the images in the dataset may also contain large number of distractor objects, as shown by the first and last images.
\newline
\newline
\section{Qualitative Results on FSC-147 Dataset}\label{dataset-images-quali}
Next, we present qualitative results on our FSC-147 dataset obtained using FamNet. For this experiment, FamNet is trained on the training set of our dataset, and we present the predicted density maps on few images from the validation and test sets. We perform test time adaptation using three exemplars, as described in the main paper.
\newline
\newline
In \Fref{fig:Qualitative4}, we present the results on few images from the validation set. We show the query image along with the exemplars shown by red bounding boxes, the groundtruth density map and predicted density map obtained by FamNet after test time adaptation. The first four query images are success cases for FamNet, while the fifth one is a failure case. The fifth image is an extremely dense image with the ground truth count of over 900. Furthermore, the object of interest is small in size. As a result, FamNet performs poorly on this query image.
\newline
\newline

In \Fref{fig:Qualitative3}, we present the qualitative results on few images from the test set. We show the query image along with the exemplars shown by red bounding boxes, the groundtruth density map and predicted density map obtained by FamNet after test time adaptation. The first three query images are success cases for FamNet, while the last two are failure cases. The fifth image is rather challenging since there is large variation in the scale of the object of interest because of perspective distortion. 
\newcommand\Aqualexheight{0.61\textwidth}

%%%%%%%%%%%%%%%%%%%%%%%%%%%%%%%%%%%%%%%%%%%%%%%%%%%%%%%%%%%
%%%%%%%%%%%%%%%%%%%%%%%%%%%%%%%%%%%%%%%%%%%%%%%%%%%%%%%%%%%%%%%
\begin{figure*}[!b]

  \begin{subfigure}[b]{0.32\textwidth}    \includegraphics[height=\Aqualexheight,width=\textwidth]{./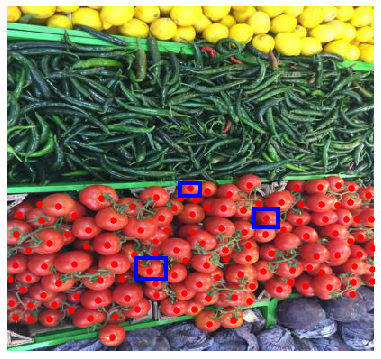}
    % \caption{Dot Annotation.}
    % \label{fig:chairs_dot}
  \end{subfigure}
  \hfill
  \begin{subfigure}[b]{0.32\textwidth}    \includegraphics[height=\Aqualexheight,width=\textwidth]{./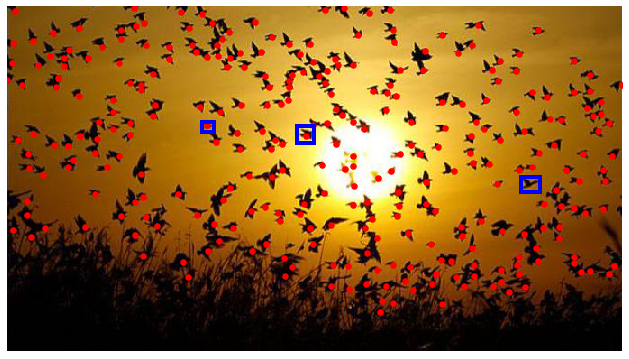}
    % \caption{Dot Annotation.}
    % \label{fig:chairs_dot}
  \end{subfigure}
  \hfill
    \begin{subfigure}[b]{0.32\textwidth}    \includegraphics[height=\Aqualexheight,width=\textwidth]{./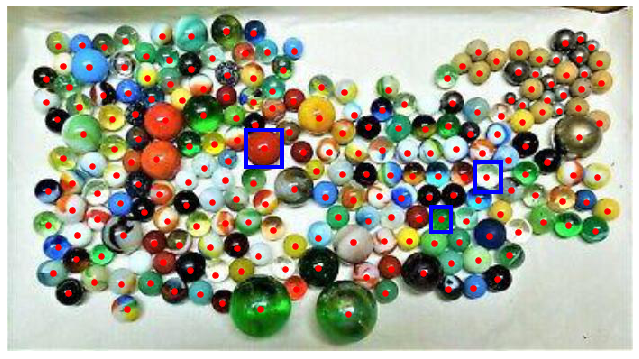}
    % \caption{Dot Annotation.}
    % \label{fig:chairs_dot}
  \end{subfigure}
  \vspace{3pt}

  \begin{subfigure}[b]{0.32\textwidth}    \includegraphics[height=\Aqualexheight,width=\textwidth]{./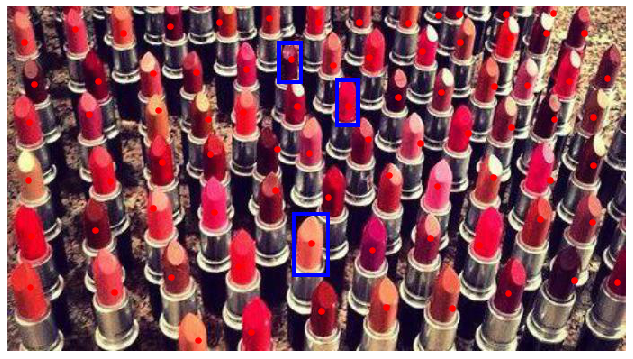}
    % \caption{Dot Annotation.}
    % \label{fig:chairs_dot}
  \end{subfigure}
  \hfill
  \begin{subfigure}[b]{0.32\textwidth}    \includegraphics[height=\Aqualexheight,width=\textwidth]{./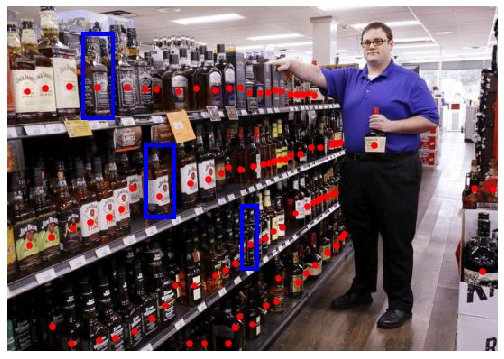}
    % \caption{Dot Annotation.}
    % \label{fig:chairs_dot}
  \end{subfigure}
  \hfill
    \begin{subfigure}[b]{0.32\textwidth}    \includegraphics[height=\Aqualexheight,width=\textwidth]{./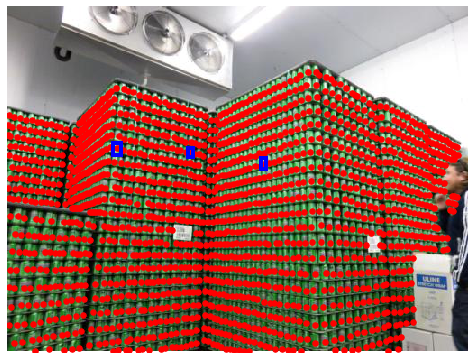}
    % \caption{Dot Annotation.}
    % \label{fig:chairs_dot}
  \end{subfigure}
  \vspace{3pt}
 
    \begin{subfigure}[b]{0.32\textwidth}    \includegraphics[height=\Aqualexheight,width=\textwidth]{./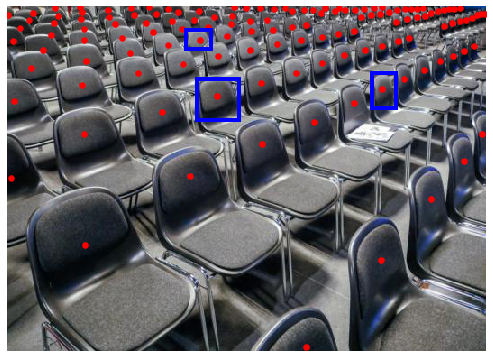}
    % \caption{Dot Annotation.}
    % \label{fig:chairs_dot}
  \end{subfigure}
  \hfill
  \begin{subfigure}[b]{0.32\textwidth}    \includegraphics[height=\Aqualexheight,width=\textwidth]{./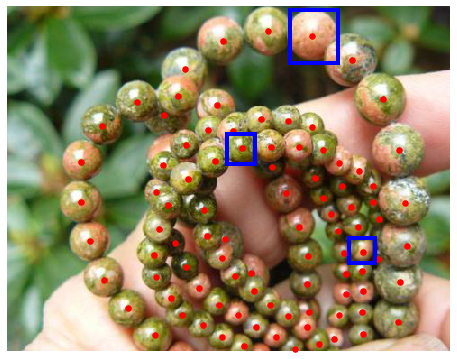}
    % \caption{Dot Annotation.}
    % \label{fig:chairs_dot}
  \end{subfigure}
  \hfill
    \begin{subfigure}[b]{0.32\textwidth}    \includegraphics[height=\Aqualexheight,width=\textwidth]{./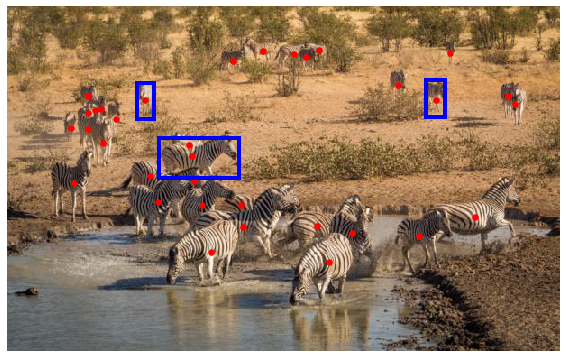}
    % \caption{Dot Annotation.}
    % \label{fig:chairs_dot}
  \end{subfigure}
  \vspace{3pt}

    \begin{subfigure}[b]{0.32\textwidth}    \includegraphics[height=\Aqualexheight,width=\textwidth]{./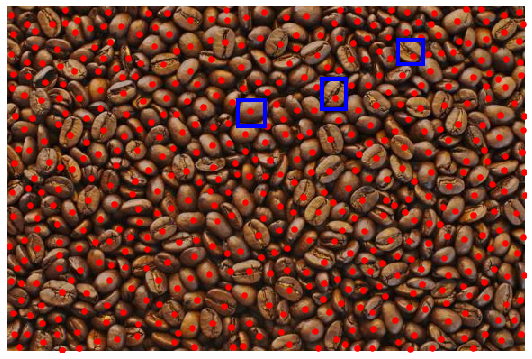}
    % \caption{Dot Annotation.}
    % \label{fig:chairs_dot}
  \end{subfigure}
  \hfill
  \begin{subfigure}[b]{0.32\textwidth}    \includegraphics[height=\Aqualexheight,width=\textwidth]{./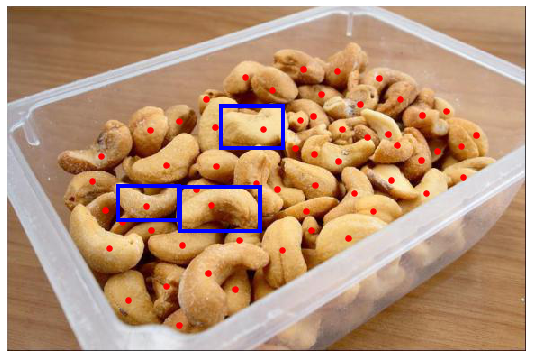}
    % \caption{Dot Annotation.}
    % \label{fig:chairs_dot}
  \end{subfigure}
  \hfill
    \begin{subfigure}[b]{0.32\textwidth}    \includegraphics[height=\Aqualexheight,width=\textwidth]{./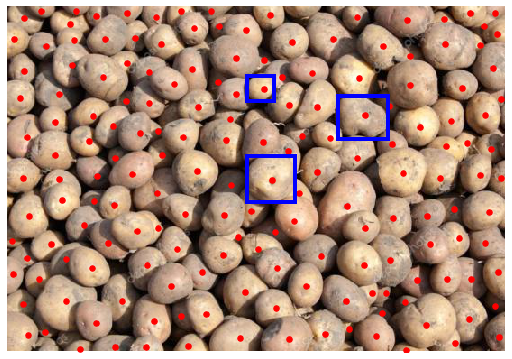}
    % \caption{Dot Annotation.}
    % \label{fig:chairs_dot}
  \end{subfigure}
  \vspace{3pt}

    \begin{subfigure}[b]{0.32\textwidth}    \includegraphics[height=\Aqualexheight,width=\textwidth]{./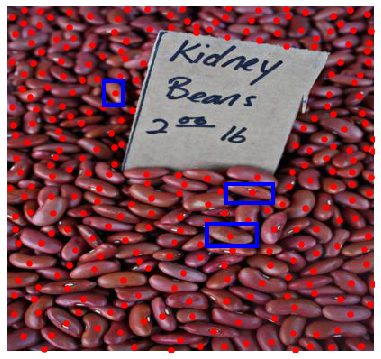}
    % \caption{Dot Annotation.}
    % \label{fig:chairs_dot}
  \end{subfigure}
  \hfill
  \begin{subfigure}[b]{0.32\textwidth}    \includegraphics[height=\Aqualexheight,width=\textwidth]{./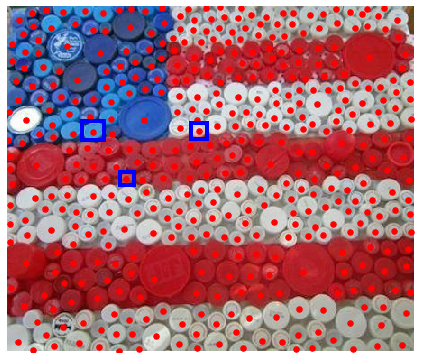}
    % \caption{Dot Annotation.}
    % \label{fig:chairs_dot}
  \end{subfigure}
  \hfill
    \begin{subfigure}[b]{0.32\textwidth}    \includegraphics[height=\Aqualexheight,width=\textwidth]{./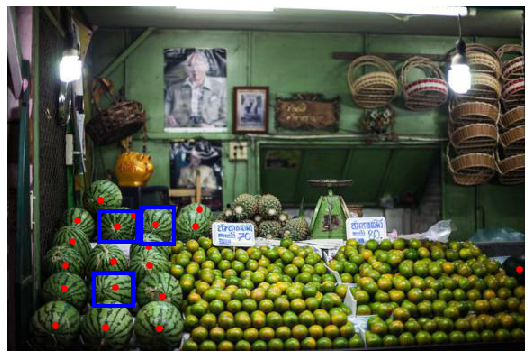}
    % \caption{Dot Annotation.}
    % \label{fig:chairs_dot}
  \end{subfigure}

  %\vspace{3pt}
%   \vspace{3pt}
\vskip -0.05in
  \caption{{\bf Few annotated images from the proposed FSC-147 dataset}. Dot and box annotations are shown in red and blue respectively. The number of objects in each image varies widely, some images contain a dozen of objects while some contains thousands.  \label{fig:annotation_examples1} }

\end{figure*}

%%%%%%%%%%%%%%%%%%%%%%%%%%%%%%%%%%%%%%%%%%%%%%%
\newcommand\qualexfour{4.1cm}
\newcommand\qualexfive{3cm}

\begin{figure*}[!hbp]  
\centering
\makebox[\qualexfour]{Image}  \hspace{.3cm}
\makebox[\qualexfour]{GT} \hspace{.3cm}
\makebox[\qualexfour]{Prediction} 
\\
    \includegraphics[width=\qualexfour,height=\qualexfive]{Images/Quali1/217.png} \hspace{.3cm}
    \includegraphics[width=\qualexfour,height=\qualexfive]{Images/Quali1/217_gt.png}  \hspace{.3cm}
        \includegraphics[width=\qualexfour,height=\qualexfive]{Images/Quali1/217_pred_adapt.png}\\    
    % \makebox[\qualextwo]{(a) Input image}
\makebox[\qualexfour]{}
\makebox[\qualexfour]{GT Count: 60} 
\makebox[\qualexfour]{Pred Count: 63}\\ \vspace{2ex}

    \includegraphics[width=\qualexfour,height=\qualexfive]{Images/Quali1/808.png} \hspace{.3cm}
    \includegraphics[width=\qualexfour,height=\qualexfive]{Images/Quali1/808_gt.png}  \hspace{.3cm}
        \includegraphics[width=\qualexfour,height=\qualexfive]{Images/Quali1/808_pred_adapt.png}\\    
    % \makebox[\qualextwo]{(a) Input image}
\makebox[\qualexfour]{}
\makebox[\qualexfour]{GT Count: 182} 
\makebox[\qualexfour]{Pred Count: 175}\\ \vspace{2ex}

    \includegraphics[width=\qualexfour,height=\qualexfive]{Images/Quali1/979.png} \hspace{.3cm}
    \includegraphics[width=\qualexfour,height=\qualexfive]{Images/Quali1/979_gt.png}  \hspace{.3cm}
        \includegraphics[width=\qualexfour,height=\qualexfive]{Images/Quali1/979_pred_adapt.png}\\    
    % \makebox[\qualextwo]{(a) Input image}
\makebox[\qualexfour]{}
\makebox[\qualexfour]{GT Count: 108} 
\makebox[\qualexfour]{Pred Count: 100}\\ \vspace{2ex}

    \includegraphics[width=\qualexfour,height=\qualexfive]{Images/Quali1/7265.png} \hspace{.3cm}
    \includegraphics[width=\qualexfour,height=\qualexfive]{Images/Quali1/7265_gt.png}  \hspace{.3cm}
        \includegraphics[width=\qualexfour,height=\qualexfive]{Images/Quali1/7265_pred_adapt.png}\\    
    % \makebox[\qualextwo]{(a) Input image}
\makebox[\qualexfour]{}
\makebox[\qualexfour]{GT Count: 47} 
\makebox[\qualexfour]{Pred Count: 42}\\ \vspace{2ex}

    \includegraphics[width=\qualexfour,height=\qualexfive]{Images/Quali1/6969_image.png} \hspace{.3cm}
    \includegraphics[width=\qualexfour,height=\qualexfive]{Images/Quali1/6969_gt.png}  \hspace{.3cm}
        \includegraphics[width=\qualexfour,height=\qualexfive]{Images/Quali1/6969_pred_adapt.png}\\    
    % \makebox[\qualextwo]{(a) Input image}
\makebox[\qualexfour]{}
\makebox[\qualexfour]{GT Count: 949} 
\makebox[\qualexfour]{Pred Count: 571}\\ \vspace{2ex}
  \vskip -0.1in
  \caption{{\bf Predicted density maps and counts of FamNet on the Validation Set of FSC-147 dataset}. Shown are query images, groundtruth maps and predicted density maps. FamNet performs well on the first four test cases, but fails on the last one. }
  \label{fig:Qualitative4}
\end{figure*}

\begin{figure*}[!thbp]  
\centering
\makebox[\qualexfour]{Image}  \hspace{.3cm}
\makebox[\qualexfour]{GT} \hspace{.3cm}
\makebox[\qualexfour]{Prediction} 
\\
    \includegraphics[width=\qualexfour,height=\qualexfive]{Images/Quali1/6809.png} \hspace{.3cm}
    \includegraphics[width=\qualexfour,height=\qualexfive]{Images/Quali1/6809_gt.png}  \hspace{.3cm}
        \includegraphics[width=\qualexfour,height=\qualexfive]{Images/Quali1/6809_pred_adapt.png}\\    
    % \makebox[\qualextwo]{(a) Input image}
\makebox[\qualexfour]{}
\makebox[\qualexfour]{GT Count: 128} 
\makebox[\qualexfour]{Pred Count: 140}\\ \vspace{2ex}

    \includegraphics[width=\qualexfour,height=\qualexfive]{Images/Quali1/309.png} \hspace{.3cm}
    \includegraphics[width=\qualexfour,height=\qualexfive]{Images/Quali1/309_gt.png}  \hspace{.3cm}
        \includegraphics[width=\qualexfour,height=\qualexfive]{Images/Quali1/309_pred_adapt.png}\\    
    % \makebox[\qualextwo]{(a) Input image}
\makebox[\qualexfour]{}
\makebox[\qualexfour]{GT Count: 113} 
\makebox[\qualexfour]{Pred Count: 96}\\ \vspace{2ex}

    \includegraphics[width=\qualexfour,height=\qualexfive]{Images/Quali1/5807.png} \hspace{.3cm}
    \includegraphics[width=\qualexfour,height=\qualexfive]{Images/Quali1/5807_gt.png}  \hspace{.3cm}
        \includegraphics[width=\qualexfour,height=\qualexfive]{Images/Quali1/5807_pred_adapt.png}\\    
    % \makebox[\qualextwo]{(a) Input image}
\makebox[\qualexfour]{}
\makebox[\qualexfour]{GT Count: 110} 
\makebox[\qualexfour]{Pred Count: 132}\\ \vspace{2ex}

    \includegraphics[width=\qualexfour,height=\qualexfive]{Images/Quali1/4291.png} \hspace{.3cm}
    \includegraphics[width=\qualexfour,height=\qualexfive]{Images/Quali1/4291_gt.png}  \hspace{.3cm}
        \includegraphics[width=\qualexfour,height=\qualexfive]{Images/Quali1/4291_pred_adapt.png}\\    
    % \makebox[\qualextwo]{(a) Input image}
\makebox[\qualexfour]{}
\makebox[\qualexfour]{GT Count: 323} 
\makebox[\qualexfour]{Pred Count: 401}\\ \vspace{2ex}

    \includegraphics[width=\qualexfour,height=\qualexfive]{Images/Quali1/2159.png} \hspace{.3cm}
    \includegraphics[width=\qualexfour,height=\qualexfive]{Images/Quali1/2159_gt.png}  \hspace{.3cm}
        \includegraphics[width=\qualexfour,height=\qualexfive]{Images/Quali1/2159_pred_adapt.png}\\    
    % \makebox[\qualextwo]{(a) Input image}
\makebox[\qualexfour]{}
\makebox[\qualexfour]{GT Count: 621} 
\makebox[\qualexfour]{Pred Count: 245}\\ \vspace{2ex}

  \vskip -0.1in
  \caption{{\bf Predicted density maps and counts of FamNet on the Test Set of FSC-147 dataset}. Shown are query images, groundtruth maps and predicted density maps. FamNet performs well on the first three test cases, but fails on the last two. }
  \label{fig:Qualitative3}
\end{figure*}

%%%%%%%%%%%%%%%%%%%%%%%%%%%%%%%%%%%%%%%%%%%%%
